# Supplementary material for: Generating Sparse Counterfactual Explanations For Multivariate Time Series
Source: arXiv:2206.00931 source file (2022-07-04)
Supplement: Supplementary file 2 [file defs.tex]

% ----------------------------------------------------------------
% General definitions
% ----------------------------------------------------------------
\renewcommand{\vec}[1]{\mathbf{#1}}


% ----------------------------------------------------------------
% Paper specific definitions
% ----------------------------------------------------------------

\newcommand{\query}{\vec{x}_{q}}
\newcommand{\target}{\vec{x}_{t}}
\newcommand{\targetclass}{\vec{c}_{t}}
\newcommand{\residuals}{\vec{\delta}}
\newcommand{\cf}{\vec{x}_{cf}}
\newcommand{\gen}{\mathcal{G}}
\newcommand{\disc}{\mathcal{D}}
\newcommand{\cls}{\mathcal{C}}
\newcommand{\genloss}{\mathcal{L}_{G}}
\newcommand{\discloss}{\mathcal{L}_{D}}
\newcommand{\advloss}{\mathcal{L}_{adv}}
\newcommand{\clsloss}{\mathcal{L}_{cls}}
\newcommand{\simloss}{\mathcal{L}_{sim}}
\newcommand{\sparseloss}{\mathcal{L}_{sparse}}
\newcommand{\jerkloss}{\mathcal{L}_{jerk}}
\newcommand{\lone}{\mathcal{L}_{1}}
\newcommand{\lzero}{\mathcal{L}_{0}}
\newcommand{\ltwo}{\mathcal{L}_{2}}
\newcommand{\ours}{SPARCE} % usage \ours{}
